# Supplementary material for: Balancing the Norwegian regulated power market anno 2016 to 2022
Source: arXiv:2402.09134 source file (2024-02-14)
Supplement: Supplementary file 1 [file appendix.tex]

\section{Supplementary figures} \label{sec:supplementary}

\begin{figure*}
    \centering
    \includegraphics[width=0.8\textwidth]{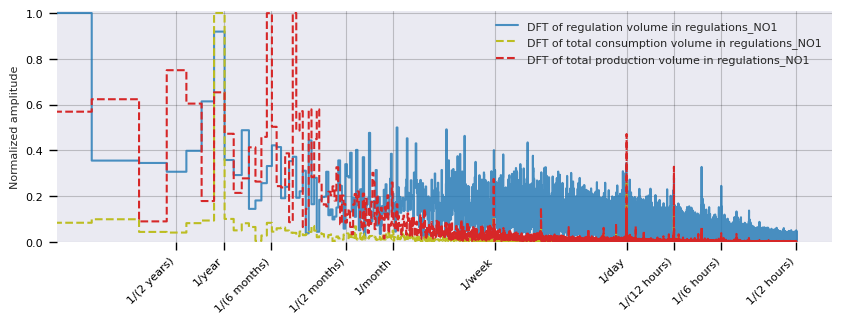}
    \includegraphics[width=0.8\textwidth]{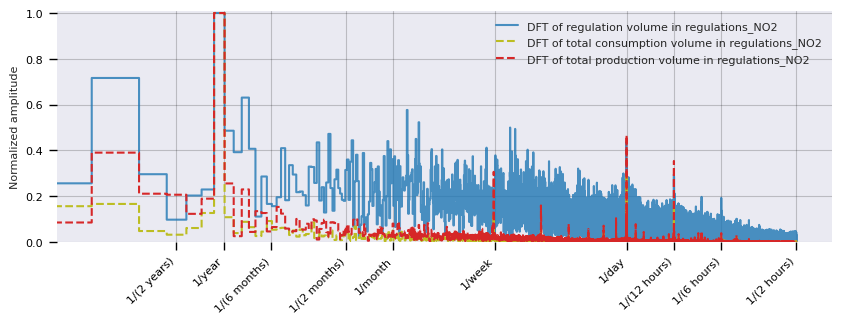}
    \includegraphics[width=0.8\textwidth]{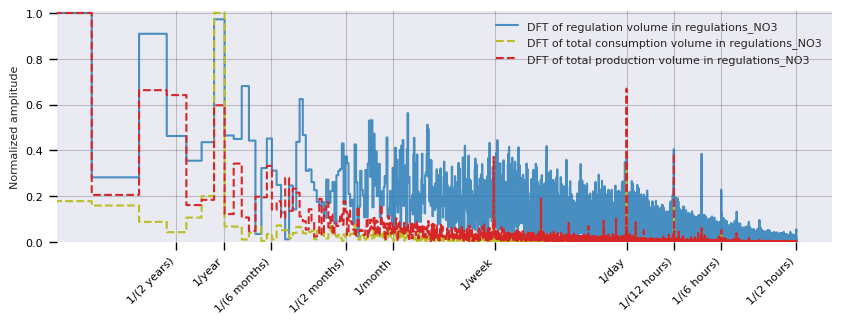}
    \includegraphics[width=0.8\textwidth]{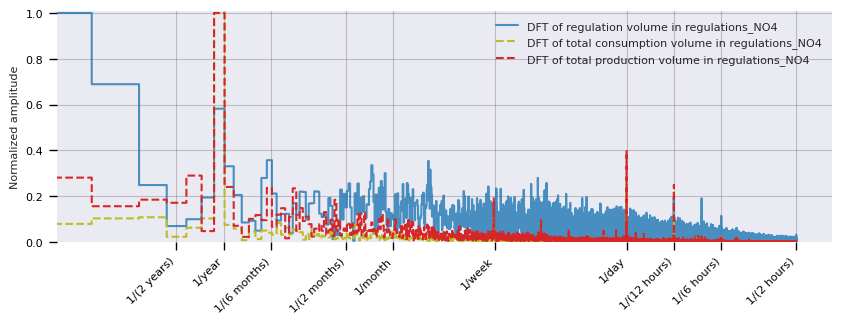}
    \caption{Discrete Fourier transform of regulation, consumption and production volumes for 2016-2022. The amplitudes are normalized to largest observed frequency spike.}
    \label{fig:app_regulation_volume_DFT}
\end{figure*}
